# Supplementary material for: Learning Diverse Options via InfoMax Termination Critic
Source: arXiv:2010.02756 source file (2023-05-31)
Supplement: Supplementary file 1 [file a-chain.tex]

\section{InfoMax Options in Deterministic Chain}
\label{appendix:chain}

\begin{figure}[t]
  \centering
  \begin{subfigure}[t]{6.8cm}
    \includegraphics[width=6.5cm]{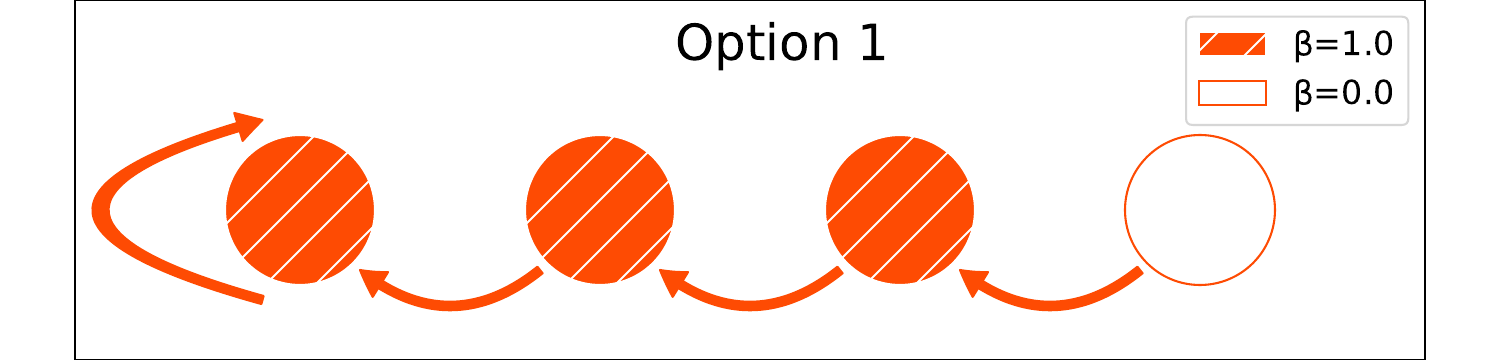}
    \includegraphics[width=6.5cm]{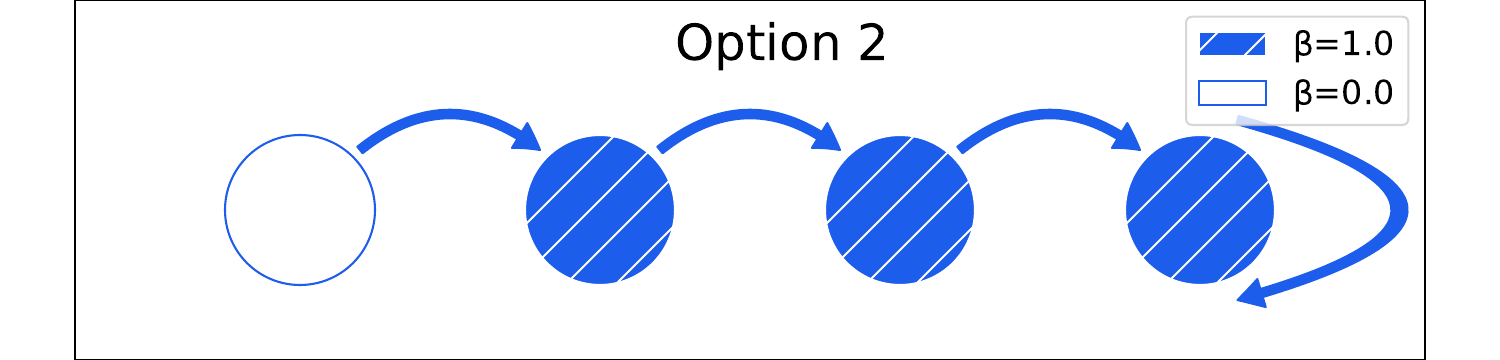}
  \end{subfigure}
  \begin{subfigure}[t]{6.8cm}
    \includegraphics[width=6.5cm]{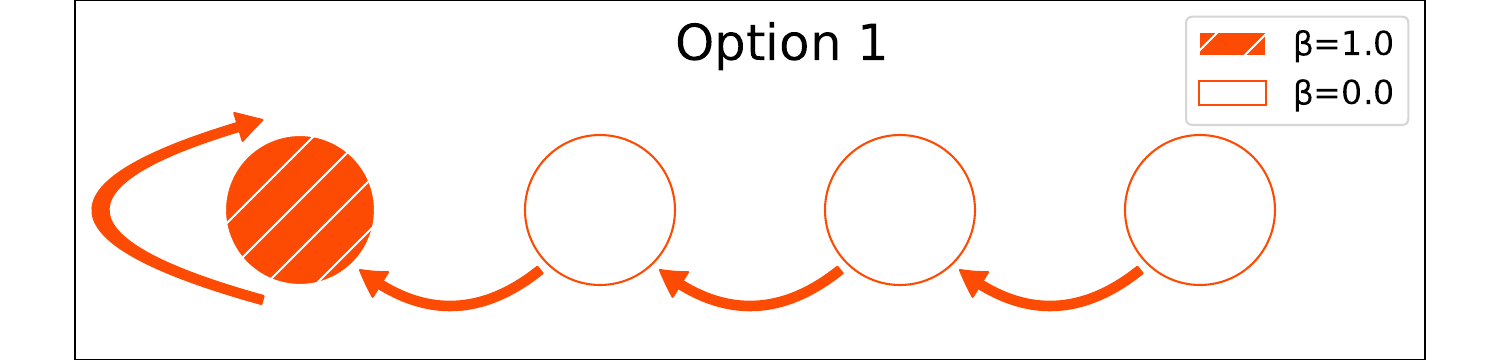}
    \includegraphics[width=6.5cm]{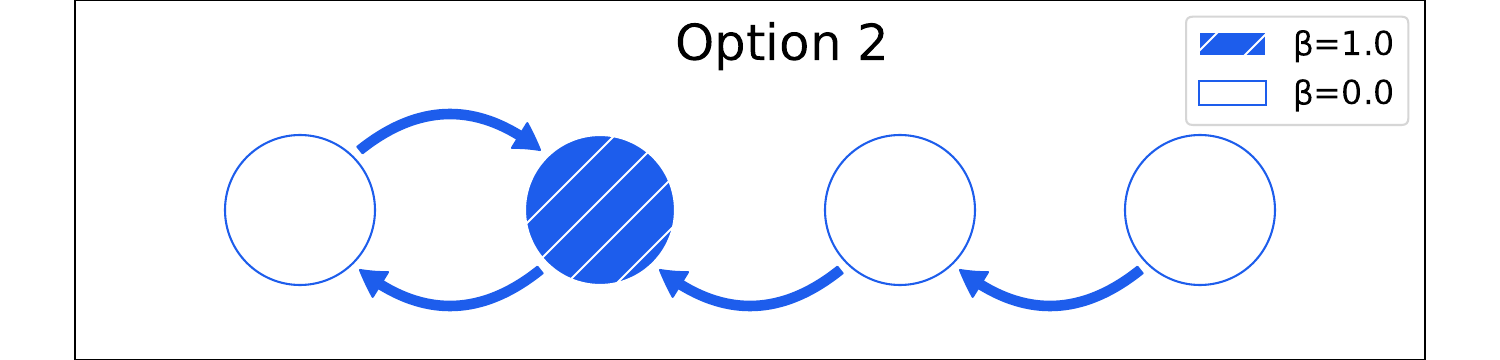}
  \end{subfigure}
  \caption{
    Two instances of InfoMax options in the four-state deterministic chain.
    \textbf{Left:} Options are diverse, but all state transitions per option are one-step.
    \textbf{Right:} Options enable relatively long state transitions, but intra-option policies are the same in some states.
  }
  \label{figure:opt2-chain}
\end{figure}

To illustrate the limitation of infomax options, we analyzed a toy four-state \textit{deterministic chain} environment, which has four states and two deterministic actions (left and right) per each state.
Deriving the exact solution is difficult, and thus, we only considered deterministic options with a minimum $H(X_f|x_s, O)$ and maximize $H(X_f|x_s)$.
Among the multiple solutions, we show two interesting deterministic infomax options when $|\Op| = 2$ in \Cref{figure:opt2-chain}.
The left options enable diverse behaviors per state, although they fail to capture long-term behaviors that are generally favorable in the literature (e.g., \citet{Mann2015AVI}).
Conversely, the right options enable relatively long, two- or three-step transitions while policies are the same in three states.
Furthermore, we can see that the two options form a small loop between the leftmost two states.
As this example shows, a major caveat of this MI-based approximation of diversity is the inability to consider the distance between states.
Therefore, neighboring states can be assigned to different groups, resulting in short options that are often undesirable.
While we do not observe such short options in \Cref{section:experiments: intrinsic} with Euclidian state spaces, this can still be problematic in general.

\begin{figure}[t]
  \centering
  \begin{subfigure}[t]{6.8cm}
    \includegraphics[width=6.5cm]{figures/chains/opt2-case2-1.pdf}
    \includegraphics[width=6.5cm]{figures/chains/opt2-case2-2.pdf}
    \includegraphics[width=6.5cm]{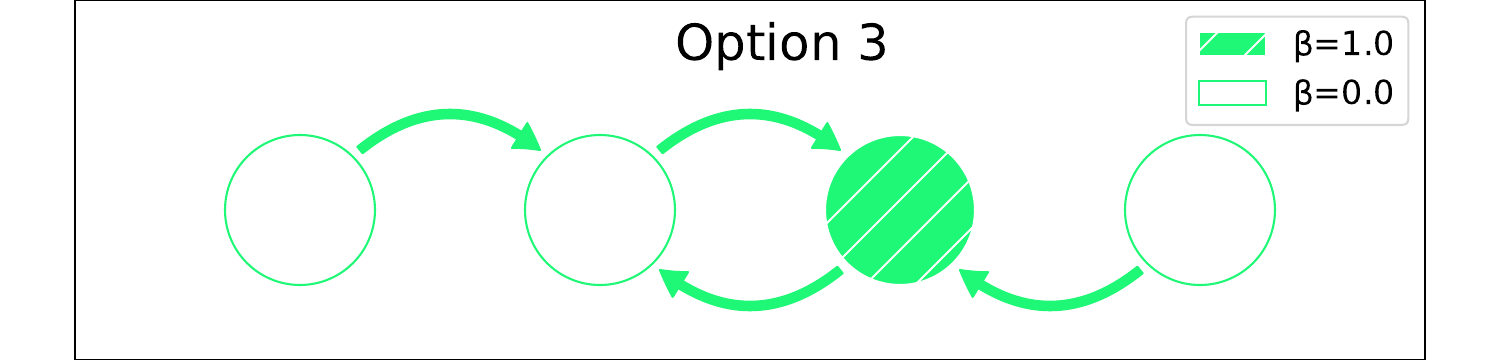}
  \end{subfigure}
  \begin{subfigure}[t]{6.8cm}
    \includegraphics[width=6.5cm]{figures/chains/opt2-case2-1.pdf}
    \includegraphics[width=6.5cm]{figures/chains/opt2-case2-2.pdf}
    \includegraphics[width=6.5cm]{figures/chains/opt3-case1-3.pdf}
    \includegraphics[width=6.5cm]{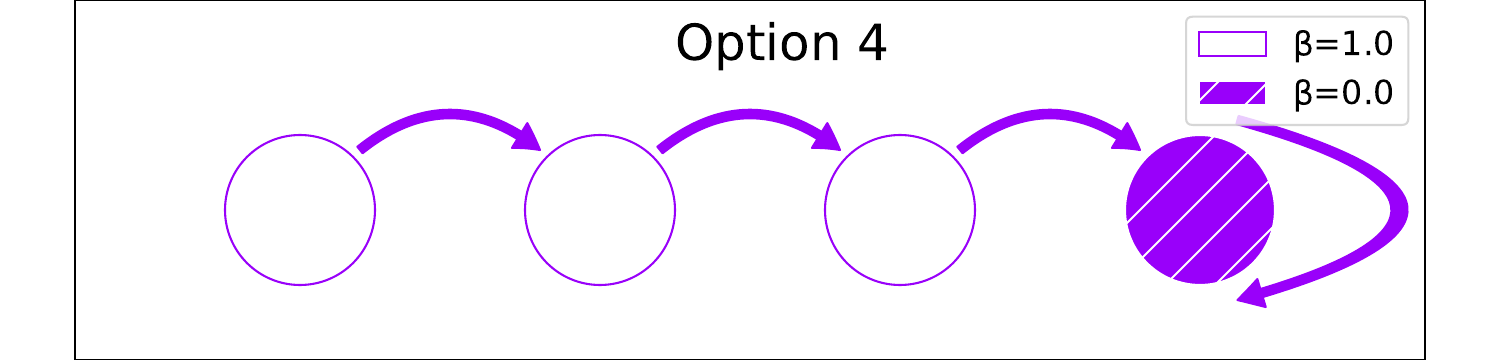}
  \end{subfigure}
  \caption{
     InfoMax options in the four state deterministic chain.
     \textbf{Left: } With three options.
     \textbf{Right: } With four options.
  }
  \label{figure:opt3-4-chain}
\end{figure}
\Cref{figure:opt3-4-chain} shows deterministic infomax options when $|\Op| = 3$ and when $|\Op| = 4$.
Among multiple solutions, we selected options with an absorbing state per option (i.e., $\bo(x) = 1.0$ for only one $x$), which are partially the same as the right options in \Cref{figure:opt2-chain}.
With four options, $\Pr(x_f|x_s) = 0.25$ for all $x_f$ and $x_s$, thus $H(X_f|x_s)$ is the maximum for all $x_s$.
This example suggests that we need as many options as the number of states to ensure that the short-cycle problem would not happen.
